# Supplementary material for: Benchmarking Differentially Private Synthetic Data Generation Algorithms
Source: arXiv:2112.09238 source file (2022-02-15)
Supplement: Supplementary file 1 [file appendix.tex]

\section{Metric Issues}

We have identified issues with several metrics we considered using

\begin{enumerate}
    \item BNLogLikelihood - favors mechanisms that generate a single very likely item, rather than capturing the full distribution well.
    \item PMSE - One weird thing about pMSE is that it doesn't seem to depend on how good the classifier is, only how good it thinks it is.  We will have a poor pMSE if the classifier predicts probabilities of 0 and 1 for every synthetic/real point, even if those predictions are completely wrong
    \item ML Efficacy metric - SDGym does not do a train/test split for this.  Favors mechanisms/ML models that overfit.
\end{enumerate}

\section{Mechanism Errors}

We now show the stack trace corresponding to mechanisms that failed in some settings.  

\subsection{FEM}
\begin{footnotesize}

\textbf{Error Key: gurobipy.GurobiError: Model too large for size-limited license;}
\begin{verbatim}
Process Process-9:
Traceback (most recent call last):
  File "/home/ubuntu/miniconda3/envs/sdg-bench/lib/python3.7/multiprocessing/process.py", line 297, in _bootstrap
    self.run()
  File "/home/ubuntu/miniconda3/envs/sdg-bench/lib/python3.7/multiprocessing/process.py", line 99, in run
    self._target(*self._args, **self._kwargs)
  File "/home/ubuntu/benchmark/tumult/synthetic-data-benchmark/mechanisms/fem_core/fem.py", line 18, in gen_fake_data
    x = oracle_weighted.solve(query_matrix, q_weigths, neg_query_matrix, n_weights, noise[i, :], domain, alpha)
  File "/home/ubuntu/benchmark/tumult/synthetic-data-benchmark/mechanisms/fem_core/Util/oracle_weighted.py", line 61, in solve
    model.optimize()
  File "src/gurobipy/model.pxi", line 847, in gurobipy.Model.optimize
gurobipy.GurobiError: Model too large for size-limited license; visit https://www.gurobi.com/free-trial for a full license
2021-08-25 16:40:18,678 : MainThread : ERROR : Error running FEM(0.100000) on dataset EchoNASDAQ_Noid; iteration 0
Traceback (most recent call last):
  File "/home/ubuntu/miniconda3/envs/sdg-bench/lib/python3.7/site-packages/sdgym/benchmark.py", line 109, in _score
    synthetic_data, model_time = _synthesize(synthesizer, real_data.copy(), metadata)
  File "/home/ubuntu/miniconda3/envs/sdg-bench/lib/python3.7/site-packages/sdgym/benchmark.py", line 42, in _synthesize
    synthetic_data = synthesizer(real_data.copy(), metadata)
  File "/home/ubuntu/benchmark/tumult/synthetic-data-benchmark/mechanisms/mechanism.py", line 60, in __call__
    synth_data = self.run(real_data)
  File "/home/ubuntu/benchmark/tumult/synthetic-data-benchmark/mechanisms/fem.py", line 86, in run
    show_prgress=True)
  File "/home/ubuntu/benchmark/tumult/synthetic-data-benchmark/mechanisms/fem_core/fem.py", line 114, in generate
    assert len(fake_temp) > 0
AssertionError
\end{verbatim}

\textbf{Error Key: Highly possibly due to same reason. The optimizer didn't work, and thus we have missing generated samples.}
\begin{verbatim}
Traceback (most recent call last):
  File "/home/ubuntu/miniconda3/envs/sdg-bench/lib/python3.7/site-packages/sdgym/benchmark.py", line 109, in _score
    synthetic_data, model_time = _synthesize(synthesizer, real_data.copy(), metadata)
  File "/home/ubuntu/miniconda3/envs/sdg-bench/lib/python3.7/site-packages/sdgym/benchmark.py", line 42, in _synthesize
    synthetic_data = synthesizer(real_data.copy(), metadata)
  File "/home/ubuntu/tumult/synthetic-data-benchmark/mechanisms/mechanism.py", line 60, in __call__
    synth_data = self.run(real_data)
  File "/home/ubuntu/tumult/synthetic-data-benchmark/mechanisms/fem.py", line 86, in run
    show_prgress=True)
  File "/home/ubuntu/tumult/synthetic-data-benchmark/mechanisms/fem_core/fem.py", line 119, in generate
    assert len(oh_fake_data) == samples, "len(D_hat) = {} len(fake_data_ = {}".format(len(oh_fake_data), len(fake_temp))
AssertionError: len(D_hat) = 36 len(fake_data_ = 36
\end{verbatim}
\end{footnotesize}

\subsection{MWEM+PGM}

\begin{footnotesize}
\begin{verbatim}
Traceback (most recent call last):
  File "/home/ubuntu/miniconda3/envs/sdg-bench/lib/python3.7/site-packages/sdgym/benchmark.py", line 109, in _score
    synthetic_data, model_time = _synthesize(synthesizer, real_data.copy(), metadata)
  File "/home/ubuntu/miniconda3/envs/sdg-bench/lib/python3.7/site-packages/sdgym/benchmark.py", line 42, in _synthesize
    synthetic_data = synthesizer(real_data.copy(), metadata)
  File "/home/ubuntu/tumult/synthetic-data-benchmark/mechanisms/mechanism.py", line 60, in __call__
    synth_data = self.run(real_data)
  File "/home/ubuntu/tumult/synthetic-data-benchmark/mechanisms/mwem.py", line 126, in run
    ax = self.worst_approximated(workload_answers, est, candidates, eps1)
  File "/home/ubuntu/tumult/synthetic-data-benchmark/mechanisms/mwem.py", line 65, in worst_approximated
    key = self.prng.choice(len(errors), p=prob)
  File "mtrand.pyx", line 928, in numpy.random.mtrand.RandomState.choice
ValueError: probabilities contain NaN
\end{verbatim}
\end{footnotesize}

\section{Note (Delete this part in the final paper)}
If we got all five runs of a specific setting missing in the result folder, it means it times out (4 hour limit). If it appears in the folder but found error message in the score file, it means RE for this setting.
